# Supplementary material for: On Grounded Planning for Embodied Tasks with Language Models
Source: arXiv:2209.00465 source file (2023-07-15)
Supplement: Supplementary file 1 [file 8_appendix.tex]

\appendix

% \section{Experimental Details}\label{sec:appendix}

\section{Full Example of Table Effect}\label{sec:full_example}

% \paragraph{Full Example in Case Study of Table Effect}

The full example is as below:
\begin{itemize}
    \item \textbf{input: } Put keys on a set of brown drawers.
    \item \textbf{truth: } STEP 1: Go to the right and stand in front of the white table. $|$ STEP 2: Pick the keys up from the table. $|$ STEP 3: Back up to face the brown drawers under the white table. $|$ STEP 4: Put the keys on top of the brown set of drawers. $|$ END
    \item \textbf{vanilla: } STEP 1: Turn left and walk to the brown drawers then turn right and walk until you're even with the black chair to your right then $|$ STEP 2: Pick up the keys that are in front of you. $|$ STEP 3: Turn around and take a step then turn left and walk to the brown drawers that are in front of you. $|$ STEP 4: Put the keys on the top right corner of the brown drawers. $|$ END
    \item \textbf{w/table: } STEP 1: Turn around, go forward to the wall, turn right, go to the desk. $|$ STEP 2: Take the keys from the desk. $|$ STEP 3: Turn around, go forward to the brown drawers. $|$ STEP 4: Put the keys on the brown drawers.  END
\end{itemize}
